# Supplementary material for: A Qualitative and Quantitative Analysis of Container Engines
Source: arXiv:2303.04080 source file (2023-03-07)
Supplement: Supplementary file 1 [file 99_appendix.tex]

\nic{Questa sezione presenta alcuni concetti che vengono utilizzati nell'articolo}

\subsection{User Namespace}
\label{subsec:user-namespace}
% user namespace
Linux containers exploit \textit{user namespaces} to work. \textit{Namespaces} provide isolation for running processes, limiting their access to system resources without the running process being aware of the limitations. The user namespace was added in Linux 3.8 and the following few releases. With a user namespace, different containers can have completely different user (uid) and group (gid) numbers. For example, a user with uid 1000 inside a container may map to user 2000 outside the container. In particular, a process can have a normal unprivileged user id outside a user namespace while at the same time having a user id of 0 inside the namespace, thus appearing to be root. This means that, the process has full privileges for operations inside the user namespace, but is unprivileged for operations outside the namespace. The \textit{user namespace} also allows a user to add/delete users inside the container.

% cgroup
\subsection{cgroup}
\label{subsec:cgroup}
The resources used by Linux containers can be limited, accounted and isolated with \textit{cgroup}. This kernel feature allows to allocate resources such as CPU time, network bandwidth and system memory to a container. Version 1 of \textit{cgroup} only supports containers that are run by root, while version 2 supports containers that are run by root or a non-privileged user.

% oci
\subsection{OCI}
\label{subsec:oci}
The Open Container Initiative (OCI) \cite{oci_website} is a Linux Foundation project to design open standards for operating-system-level virtualization, such as Linux containers. OCI containers aim to define an industry standards around container image formats and runtimes. The OCI currently contains two specifications: the Runtime Specification (runtime-spec) \cite{ociruntime_website} and the Image Specification (image-spec) \cite{ociimage_website}. Given an OCI image, any container runtime that implements the OCI Runtime Specification can unbundle the image and run its contents in an isolated environment.

% hooks
The OCI Runtime Specification allows for components to be hooked into the container's lifecycle in order to perform custom actions, allowing to extend the core functionality provided by a container runtime. OCI hooks are particularly used in the High Performance Computing (HPC) context where the dedicated hardware and highly-tuned software adopted by high-performance systems are in contrast with the platform-agnostic nature of software containers. OCI Hooks provide solutions for the container runtime to allow access to system-specific features and specialized resources within container instances.
